# Supplementary material for: FlexFL: Heterogeneous Federated Learning via APoZ-Guided Flexible Pruning in Uncertain Scenarios
Source: arXiv:2407.12729 source file (2024-07-17)
Supplement: Supplementary file 1 [file appendix.tex]

% \section{Proof of Theorem~\ref{thm:full}}
% \label{appen:full}
% We analyze \texttt{FedAvg} in the setting of full device participation in this section.

% \subsection{Additional Notation}
% Let $\w_t^k$ be the model parameter maintained in the $k$-th device at the $t$-th step. Let $\IM_E$ be the set of global synchronization steps, i.e., $\IM_E = \{nE \  | \ n=1,2,\cdots\}$. If $t+1 \in \IM_E$, i.e., the time step to communication, \texttt{FedAvg} activates all devices. Then the update of \texttt{FedAvg} with partial devices active can be described as
% \begin{align}
% & \v_{t+1}^k = \w_t^k - \eta_t \nabla F_k(\w_t^k, \xi_t^k), 
% \label{eq:update_pre}\\
% & \w_{t+1}^k =\left\{\begin{array}{ll}
% \v_{t+1}^k           & \text{ if } t+1 \notin \IM_E, \\
% \sum_{k=1}^N p_k \v_{t+1}^k   & \text{ if } t+1  \in \IM_E.
% \label{eq:ave_pre}
% \end{array}\right. 
% \end{align}
% Here, an additional variable $\v_{t+1}^k$ is introduced to represent the immediate result of one step SGD update from $\w_t^k$. We interpret $\w_{t+1}^k$ as the parameter obtained after communication steps (if possible).

% In our analysis, we define two virtual sequences $\av_t = \myave \v_t^k$ and $\aw_t = \myave \w_t^k$. This is motivated by \citep{stich2018local}. $\av_{t+1}$ results from an single step of SGD from $\aw_{t}$. 
% When $t+1 \notin \IM_E$, both are inaccessible. When $t+1 \in \IM_E$, we can only fetch $\aw_{t+1}$. For convenience, we define $\overline{\g}_t = \myave \nabla F_k(\w_t^k)$ and $\g_t = \myave \nabla F_k(\w_t^k, \xi_t^k)$.  
% Therefore, $\overline{\v}_{t+1} = \overline{\w}_t - \eta_t \g_t$ and $\EB \g_t = \overline{\g}_t$.


% \subsection{Key Lemmas}
% To convey our proof clearly, it would be necessary to prove certain useful lemmas. We defer the proof of these lemmas to latter section and focus on proving the main theorem.

% \begin{lem}[Results of one step SGD]
% \label{lem:conv_main} Assume Assumption~\ref{asm:smooth} and~\ref{asm:strong_cvx}. If $\eta_t\leq \frac{1}{4L}$, we have
% \[  
% \EB \left\|\overline{\v}_{t+1}-\w^{\star}\right\|^{2} 
% \leq (1-\eta_t \mu) \EB \left\|\overline{\w}_{t}-\w^{\star}\right\|^{2}     
% + \eta_{t}^{2} \EB \left\|\mathbf{g}_{t}-\overline{\mathbf{g}}_{t}\right\|^{2} + 6L \eta_t^2 \Gamma 
% + 2 \EB \myave \left\|\overline{\w}_{t}-\w_{k}^{t}\right\|^{2} 
% \]
% where $\Gamma = F^* - \myave F_k^{\star} \ge 0$.
% \end{lem}


% \begin{lem}[Bounding the variance]
% Assume Assumption~\ref{asm:sgd_var} holds. It follows that
% 	\label{lem:conv_variance}
% 	\[\EB \left\|\mathbf{g}_{t}-\overline{\mathbf{g}}_{t}\right\|^{2}  \leq \sum_{k=1}^N p_k^2 \sigma_k^2.\]
% \end{lem}


% \begin{lem}[Bounding the divergence of $\{\w_t^k\}$]
% 	\label{lem:conv_diversity}
% 	Assume Assumption~\ref{asm:sgd_norm}, that $\eta_t$ is non-increasing and $\eta_{t} \le 2 \eta_{t+E}$ for all $t\geq 0$. It follows that
% 	\[\EB \left[ \myave \left\|\overline{\w}_{t}-\w_{k}^{t}\right\|^{2} \right]
% 	\: \leq \: 4 \eta_t^2 (E-1)^2 G^2.\]
% \end{lem}

% \subsection{Completing the Proof of Theorem~\ref{thm:full}}
% \begin{proof}
% It is clear that no matter whether $t+1 \in \IM_E$ or $t+1 \notin \IM_E$, we always have $\aw_{t+1}= \av_{t+1}$. Let $\Delta_t=\EB \left\|\aw_{t}-\w^{\star}\right\|^{2}$. From Lemma~\ref{lem:conv_main}, Lemma~\ref{lem:conv_variance} and Lemma~\ref{lem:conv_diversity}, it follows that
% \begin{equation}
% \label{eq:conv_full_final}
% \Delta_{t+1} \le (1-\eta_t \mu) \Delta_t + \eta_t^2 B
% \end{equation}
% where
% \[ B = \sum_{k=1}^N p_k^2 \sigma_k^2 +  6L \Gamma + 8 (E-1)^2G^2. \]

%  For a diminishing stepsize, $\eta_t = \frac{\beta}{t + \gamma}$ for some $\beta > \frac{1}{\mu}$ and $\gamma > 0$ such that $\eta_1 \le \min\{\frac{1}{\mu}, \frac{1}{4L}\}=\frac{1}{4L}$ and $\eta_{t} \le 2 \eta_{t+E}$. We will prove $\Delta_t \le \frac{v}{\gamma + t}$ where $v = \max\left\{ \frac{\beta^2 B}{\beta \mu -1}, (\gamma+1)\Delta_1 \right\}$.

% We prove it by induction. Firstly, the definition of $v$ ensures that it holds for $t = 1$. Assume the conclusion holds for some $t$, it follows that
% \begin{align*}
% \Delta_{t+1} 
% &\le (1-\eta_t\mu )\Delta_t + \eta_t^2 B \\
% &\le \left(1- \frac{\beta\mu}{t + \gamma}\right)\frac{v}{t + \gamma} + \frac{\beta^2B}{(t + \gamma)^2}\\
% &=\frac{t + \gamma -1}{(t + \gamma)^2} v  + \left[ \frac{\beta^2B}{(t + \gamma)^2} - \frac{\beta\mu-1}{(t+\gamma)^2}v \right] \\
% & \le \frac{v}{t + \gamma +1}.
% \end{align*}

% Then by the $L$-smoothness of $F(\cdot)$,
% \[  \EB [F(\aw_t)] - F^* \le \frac{L}{2} \Delta_t  \le \frac{L}{2} \frac{v}{\gamma + t}.\]
% Specifically, if we choose $\beta = \frac{2}{\mu}, \gamma = \max\{8 \frac{L}{\mu}, E\}-1$ and denote $\kappa = \frac{L}{\mu}$, then  $\eta_t = \frac{2}{\mu} \frac{1}{\gamma + t}$.
% One can verify that the choice of $\eta_{t}$ satisfies $\eta_{t} \le 2\eta_{t+E}$ for $t \ge 1$.
% Then, we have
% \[
% v = \max\left\{ \frac{\beta^2 B}{\beta \mu -1}, (\gamma+1)\Delta_1 \right\} 
% \le \frac{\beta^2 B}{\beta \mu -1} +  (\gamma+1)\Delta_1 \le 
% \frac{4B}{\mu^2} + (\gamma+1) \Delta_1,
% \]
% and 
% \[  \EB [F(\aw_t)] - F^*
%  \le   \frac{L}{2} \frac{v}{\gamma + t} 
%  \le   \frac{\kappa}{\gamma + t} \left( \frac{2B}{\mu} +   \frac{\mu (\gamma+1)}{2} \Delta_1 \right). \]
% \end{proof}


% \subsection{Deferred proofs of key lemmas}
% \begin{proof}[Proof of Lemma~\ref{lem:conv_main}.]
% 	Notice that $\av_{t+1} = \aw_t - \eta_t \vg_t$, then
% 	\begin{align}
% 	\label{eq:partial_main}
% 	\left\|\overline{\v}_{t+1}-\w^{\star}\right\|^{2} \nonumber 
% 	&=\left\|\overline{\w}_{t}-\eta_{t} \mathbf{g}_{t}-\w^{\star}-\eta_{t} \overline{\mathbf{g}}_{t}+\eta_{t} \overline{\mathbf{g}}_{t}\right\|^{2} \nonumber \\ 
% 	&=\underbrace{\left\|\overline{\w}_{t}-\w^{\star}-\eta_{t} \overline{\mathbf{g}}_{t}\right\|^{2}}_{A_1}+
% 	\underbrace{2\eta_{t}\left\langle\overline{\w}_{t}-\w^{\star}-\eta_{t} \overline{\mathbf{g}}_{t}, \overline{\mathbf{g}}_{t}-\mathbf{g}_{t}\right\rangle}_{A_2} +
% 	\eta_{t}^{2}\left\|\mathbf{g}_{t}-\overline{\mathbf{g}}_{t}\right\|^{2}
% 	\end{align}
% 	Note that $\EB A_2 = 0$. We next focus on bounding $A_1$. Again we split $A_1$ into three terms:
% 	\begin{equation}
% 	\label{eq:partial_proof_main_term}
% 	\left\|\overline{\w}_{t}-\w^{\star}-\eta_{t} \overline{\mathbf{g}}_{t}\right\|^{2} =\left\|\overline{\w}_{t}-\w^{\star}\right\|^{2}
% 	\underbrace{-2 \eta_{t}\left\langle\overline{\w}_{t}-\w^{\star}, \overline{\mathbf{g}}_{t}\right\rangle}_{B_1}
% 	+  \underbrace{\eta_{t}^{2}\left\|\overline{\mathbf{g}}_{t}\right\|^{2}}_{B_2}
% 	\end{equation}
	
% 	From the the $L$-smoothness of $F_k(\cdot)$, it follows that
% 	\begin{equation}
% 	\label{eq:partial_proof_L}
% 	  \left\|\nabla F_k\left(\w_{t}^{k}\right)\right\|^{2} \leq 2 L\left(F_k\left(\w_{t}^{k}\right)-F_k^{\star}\right).
% 	\end{equation}
	
% 	By the convexity of $\left\| \cdot \right \|^2$ and~\eqref{eq:partial_proof_L}, we have
% 	\[
% 	B_2 = \eta_{t}^{2}\left\|\overline{\mathbf{g}}_{t}\right\|^{2} 
% 	\leq \eta_{t}^{2}\myave \left\|\nabla F_k\left(\w_{t}^{k}\right)\right\|^{2}
% 	\leq 2L\eta_t^2 \myave \left( F_k(\w_t^k) - F_k^*\right).
% 	\]
	
% 	Note that 
% 	\begin{align}
% 	\label{eq:partial_B1}
% 	  B_1 
% 	  &= -2 \eta_{t}\left\langle\overline{\w}_{t}-\w^{\star}, \overline{\mathbf{g}}_{t}\right\rangle 
% 	  = -2\eta_t \myave \left\langle\overline{\w}_{t}-\w^{\star}, \nabla F_k(\w_t^k)\right\rangle \nonumber \\
% 	  &=-2\eta_t \myave \left\langle\overline{\w}_{t}-\w_t^k, \nabla F_k(\w_t^k)\right\rangle
% 	  -2\eta_t \myave \left\langle\w_t^k-\w^{\star}, \nabla F_k(\w_t^k)\right\rangle.
% 	\end{align}
	
% 	By Cauchy-Schwarz inequality and AM-GM inequality, we have
% 	\begin{equation}
% 	\label{eq:partial_B11}
% 	-2 \left\langle\overline{\w}_{t}-\w_t^{k}, \nabla F_k \left(\w_{t}^{k}\right)\right\rangle \leq \frac{1}{\eta_t} \left\|\overline{\w}_{t}-\w_{t}^{k}\right\|^{2}
% 	+ \eta_t \left\|\nabla F_k\left(\w_{t}^{k}\right)\right\|^{2}.	
% 	\end{equation}
	
% 	By the $\mu$-strong convexity of $F_k(\cdot)$, we have
% 	\begin{equation}
% 	\label{eq:partial_B12}
% 	-\left\langle\w_{t}^{k}-\w^{\star}, \nabla F_k\left(\w_{t}^{k}\right)\right\rangle \leq -\left(F_k\left(\w_{t}^{k}\right)-F_k(\w^*)\right)-\frac{\mu}{2}\left\|\w_{t}^{k}-\w^{\star}\right\|^{2}.
% 	\end{equation}
	
% 	By combining ~\eqref{eq:partial_proof_main_term},~\eqref{eq:partial_B1},~\eqref{eq:partial_B11} and~\eqref{eq:partial_B12}, it follows that
% 	\begin{align*}
% 	 A_1 
% 	 =  \left\|\overline{\w}_{t}-\w^{\star}-\eta_{t} \overline{\mathbf{g}}_{t}\right\|^{2} 
% 	 &\leq \left\|\overline{\w}_{t}-\w^{\star}\right\|^{2} 
% 	 + 2L\eta_t^2 \myave \left( F_k(\w_t^k) - F_k^*\right) \\
% 	 & \quad +\eta_t \myave \left(\frac{1}{\eta_t} \left\|\overline{\w}_{t}-\w_{k}^{t}\right\|^{2}+\eta_t \left\|\nabla F_k\left(\w_{t}^{k}\right)\right\|^{2}\right)  \\ 
% 	&  \quad -2\eta_t \myave \left( F_k\left(\w_{t}^{k}\right)-F_k(\w^*) + \frac{\mu}{2}\left\|\w_{t}^{k}-\w^{\star}\right\|^{2} \right) \\
% 	& = (1-\mu\eta_t)\left\|\overline{\w}_{t}-\w^{\star}\right\|^{2} 
% 	+ \myave \left\|\overline{\w}_{t}-\w_{k}^{t}\right\|^{2} \\
% 	& \quad + \underbrace{4L\eta_t^2 \myave \left( F_k(\w_t^k) - F_k^*\right) 
% 	 - 2\eta_t \myave \left(F_k\left(\w_{t}^{k}\right)-F_k(\w^*)\right)}_{C}
% 	\end{align*}
% 	where we use~\eqref{eq:partial_proof_L} again.
	
	
% 	We next aim to bound $C$. We define $\gamma_t = 2\eta_t(1-2L\eta_t)$. Since $\eta_t \leq \frac{1}{4L}$, $\eta_t \le \gamma_t \leq 2\eta_t$. Then we split $C$ into two terms:
% 	\begin{align*}
% 	 C &= - 2\eta_t(1-2L\eta_t) \myave \left( F_k(\w_t^k) - F_k^* \right) 
% 	 + 2\eta_t \myave \left(F_k(\w^*) - F_k^*\right) \\
% 	 &=-\gamma_t \myave \left( F_k(\w_t^k) - F^* \right)  
% 	  + (2\eta_t-\gamma_t)\myave  \left( F^*-F_k^*\right)  \\
% 	 &=\underbrace{-\gamma_t \myave \left( F_k(\w_t^k) - F^* \right)}_{D}
% 	 +4L\eta_t^2 \Gamma
% 	\end{align*}
% 	where in the last equation, we use the notation $\Gamma = \myave \left( F^*-F_k^*\right)=F^* - \myave F_k^*$.
	
% 	To bound $D$, we have
% 	\begin{align*}
% 	\myave \left( F_k(\w_t^k) - F^*  \right)
% 	 &=\myave \left( F_k(\w_t^k) - F_k(\overline{\w}_t)  \right) 
% 	 + \myave \left( F_k(\overline{\w}_t) - F^*  \right)\\
% 	 & \ge \myave\left\langle \nabla F_k(\overline{\w}_t), \overline{\w}_t^k - \overline{\w}_t \right\rangle
% 	 + \left( F(\aw_t) - F^* \right) \\
% 	 & \ge - \frac{1}{2} \myave \left[ \eta_t\left\|  \nabla F_k(\overline{\w}_t) \right\|^2 + \frac{1}{\eta_t}\left\|\w_t^k -\overline{\w}_t\right\|^2 \right]
% 	 + \left( F(\aw_t) - F^* \right) \\
% 	 & \ge - \myave \left[ \eta_tL \left(F_k(\overline{\w}_t) -F_k^*   \right)
% 	 + \frac{1}{2\eta_t}\left\|\w_t^k -\overline{\w}_t\right\|^2 \right]
% 	 + \left( F(\aw_t) - F^* \right)
% 	\end{align*}
% 	where the first inequality results from the convexity of $F_k(\cdot)$, the second inequality from AM-GM inequality and the third inequality from~\eqref{eq:partial_proof_L}.
	
% 	Therefore 
% 	\begin{align*}
% 	  C 
% 	 &= \gamma_t \myave \left[ \eta_tL \left(F_k(\overline{\w}_t) -F_k^*   \right)
% 	 + \frac{1}{2\eta_t}\left\|\w_t^k -\overline{\w}_t\right\|^2 \right]
% 	 - \gamma_t \left( F(\aw_t) - F^* \right) + 4L\eta_t^2 \Gamma\\
% 	 &= \gamma_t(\eta_t L -1 ) \myave \left(F_k(\aw_t) -F^* \right)
% 	 + \left( 4L\eta_t^2 + \gamma_t\eta_tL \right) \Gamma + \frac{\gamma_t}{2\eta_t } \myave \left\|\w_t^k -\overline{\w}_t\right\|^2 \\
% 	 &\le 6L\eta_t^2 \Gamma
%      + \myave \left\|\w_t^k -\overline{\w}_t\right\|^2 
% 	\end{align*}
% 	where in the last inequality, we use the following facts: (1) $\eta_t L -1 \le - \frac{3}{4} \le 0$ and  $\myave \left(F_k(\aw_t) -F^* \right) = F(\aw_t) - F^*\ge 0$ (2) $\Gamma \ge 0$ and $4L\eta_t^2 + \gamma_t\eta_tL \le 6\eta_t^2L$ and (3) $\frac{\gamma_t}{2\eta_t} \le 1$.
	
% 	Recalling the expression of $A_1$ and plugging $C$ into it, we have
% 	\begin{align}
% 	\label{eq:partial_proof_A1}
% 	  A_1 
% 	  &= \left\|\overline{\w}_{t}-\w^{\star}-\eta_{t} \overline{\mathbf{g}}_{t}\right\|^{2} \nonumber\\
%       &\le (1-\mu\eta_t)\left\|\overline{\w}_{t}-\w^{\star}\right\|^{2} 
% 	  + 2 \myave \left\|\overline{\w}_{t}-\w_{k}^{t}\right\|^{2} + 6\eta_t^2L \Gamma 
% 	\end{align}
% 	Using~\eqref{eq:partial_proof_A1} and taking expectation on both sides of~\eqref{eq:partial_main}, we erase the randomness from stochastic gradients, we complete the proof.
% \end{proof}



% \begin{proof}[Proof of Lemma~\ref{lem:conv_variance}]
%     From Assumption~\ref{asm:sgd_var}, the variance of the stochastic gradients in device $k$ is bounded by $\sigma_k^2$, then
% 	\begin{align*}
% 	\EB \left\|\mathbf{g}_{t}-\overline{\mathbf{g}}_{t}\right\|^{2}  & = \EB \left\| \myave (\nabla F_k(\w_t^k,\xi_t^k) - \nabla F_k(\w_t^k))  \right\|^{2}, \\
% 	&= \myave^2 \EB \left\|  \nabla F_k(\w_t^k,\xi_t^k) - \nabla F_k(\w_t^k)  \right\|^{2}, \\
% 	& \leq \sum_{k=1}^N p_k^2 \sigma_k^2.
% 	\end{align*}
% \end{proof}


% \begin{proof}[Proof of Lemma~\ref{lem:conv_diversity}]
%     Since \texttt{FedAvg} requires a communication each $E$ steps. Therefore, for any $t \ge 0$, there exists a $t_0 \leq t$, such that $t-t_0 \leq E-1$ and $\w_{t_0}^k=\aw_{t_0}$ for all $k=1,2,\cdots,N$. Also, we use the fact that $\eta_t$ is non-increasing and $\eta_{t_0} \leq 2 \eta_t$ for all $t-t_0 \leq E-1$, then
% 	\begin{align*}
% 	\EB  \myave \left\|\overline{\w}_{t}-\w_{t}^{k}\right\|^{2} &= \EB  \myave \left\|  (\w_{t}^{k} - \aw_{t_0})  - (\overline{\w}_{t} - \aw_{t_0})   \right\|^{2} \\
% 	&\leq \EB \myave \left\|  \w_{t}^{k} - \aw_{t_0}  \right\|^{2} \\
% 	& \leq \myave \EB \sum_{t = t_0}^{t-1}(E-1) \eta_t^2 \left\|  \nabla F_k(\w_t^{k},\xi_t^k)     \right\|^2 \\
% 	& \leq \myave \sum_{t=t_0} ^{t-1} (E-1) \eta_{t_0}^2 G^2 \\
% 	& \leq \myave  \eta_{t_0}^2 (E-1)^2 G^2 \\
% 	& \leq 4 \eta_t^2 (E-1)^2 G^2.
% 	\end{align*}
% 	Here in the first inequality, we use $\EB \| X - \EB X \|^2 \le \EB \|X\|^2$ where $X = \w_t^{k} - \overline{\w}_{t_0}$ with probability $p_k$.
% 	In the second inequality, we use Jensen inequality:
% 	\[
% 	\left\|  \w_{t}^{k} - \aw_{t_0}  \right\|^{2} = 
% 	\left\|  \sum_{t=t_0}^{t-1} \eta_{t}  \nabla F_k(\w_t^{k},\xi_t^k)    \right\|^{2}
% 	\le (t-t_0) \sum_{t=t_0}^{t-1} \eta_{t}^2 \left\|  \nabla F_k(\w_t^{k},\xi_t^k)   \right\|^2.
% 	\]
% 	In the third inequality, we use $\eta_{t} \le \eta_{t_0}$ for $t \ge t_0$ and $\EB \|\nabla F_k(\w_t^{k},\xi_t^k)  \|^2 \le G^2$ for $k=1,2,\cdots N$ and $t \ge 1$.
% 	In the last inequality, we use $\eta_{t_0} \le 2 \eta_{t_0+E} \le 2 \eta_{t}$ for $t_0 \le t \le t_0 + E$.
% \end{proof}



% \section{Proofs of Theorems~\ref{thm:w_replace} and~\ref{thm:wo_replace}}
% \label{appen:prov}

% We analyze \texttt{FedAvg} in the setting of partial device participation in this section.

% \subsection{Additional Notation}
% Recall that $\w_t^k$ is the model parameter maintained in the $k$-th device at the $t$-th step. $\IM_E = \{nE \  | \ n=1,2,\cdots\}$ is the set of global synchronization steps. Unlike the setting in Appendix~\ref{appen:full}, when it is the time to communicate, i.e., $t+1 \in \IM_E$, the scenario considered here is that \texttt{FedAvg} randomly activates a subset of devices according to some sampling schemes. Again, $\overline{\g}_t = \myave \nabla F_k(\w_t^k)$ and $\g_t = \myave F_k(\w_t^k, \xi_t^k)$.  Therefore, $\overline{\v}_{t+1} = \overline{\w}_t - \eta_t \g_t$ and $\EB \g_t = \overline{\g}_t$.


% \paragraph{Multiset selected.} 
% All sampling schemes can be divided into two groups, one with replacement and the other without replacement. For those with replacement,  it is possible for a device to be activated several times in a round of communication, even though each activation is independent with the rest. We denote by $\HM_t$ the multiset selected which allows any element to appear more than once. Note that $\HM_t$ is only well defined for $t \in \IM_E$. For convenience, we denote by $\SM_t = \HM_{N(t, E)}$ the most recent set of chosen devices where $N(t, E) = \max\{n| n \le t, n \in \IM_E\}$. 


% \paragraph{Updating scheme.}
% Limited to realistic scenarios (for communication efficiency and low straggler effect), \text{FedAvg} first samples a random multiset $\SM_t$ of devices and then only perform updates on them. This make the analysis a little bit intricate, since $\SM_t$ varies each $E$ steps. However, we can use a thought trick to circumvent this difficulty. We assume that \texttt{FedAvg} always activates \textbf{all devices} at the beginning of each round and then uses the parameters maintained in only a few sampled devices to produce the next-round parameter. It is clear that this updating scheme is equivalent to the original. Then the update of \texttt{FedAvg} with partial devices active can be described as: for all $k \in [N]$,
% \begin{align}
% & \v_{t+1}^k = \w_t^k - \eta_t \nabla F_k(\w_t^k, \xi_t^k), 
% \label{eq:partial_update_before}\\
% & \w_{t+1}^k =\left\{\begin{array}{ll}
% \v_{t+1}^k           & \text{ if } t+1 \notin \IM_E, \\
% \text{samples} \ \SM_{t+1} \text{ and average }  \{ \v_{t+1}^k\}_{k \in \SM_{t+1}}  & \text{ if } t+1  \in \IM_E.
% \label{eq:partial_update_after}
% \end{array}\right. 
% \end{align}


% \paragraph{Sources of randomness.}
% In our analysis, there are two sources of randomness. One results from the stochastic gradients and the other is from the random sampling of devices. 
% All the analysis in Appendix~\ref{appen:full} only involve the former. To distinguish them, we use the notation $\EB_{\SM_t}(\cdot)$, when we take expectation to erase the latter type of randomness. 


% \subsection{Key Lemmas}
% \paragraph{Two schemes.}
% For full device participation, we always have $\aw_{t+1} = \av_{t+1}$. This is true when $t+1 \notin \IM_E$ for partial device participation. When $t{+}1 \in \IM_E$, we hope this relation establish in the sense of expectation. To that end, we require the sampling and averaging scheme to be unbiased in the sense that
% \[  \EB_{\SM_{t+1}}  \aw_{t+1} = \av_{t+1}.  \]

% We find two sampling and averaging schemes satisfying the requirement and provide convergence guarantees.
% \begin{enumerate}[(I)]
% 	\item The server establishes $\SM_{t+1}$ by i.i.d. \textbf{with replacement} sampling an index $k \in \{1,\cdots,N\}$ with probabilities $p_1,\cdots,p_N$ for $K$ times. Hence $\SM_{t+1}$ is a multiset which allows a element to occur more than once. Then the server averages the parameters by $\w_{t+1}^k  = \frac{1}{K} \sum_{k \in \SM_{t+1}} \v_{t+1}^k$. This is first proposed in \citep{sahu2018convergence} but lacks theoretical analysis.
% 	\item The server samples $\SM_{t+1}$ uniformly in a \textbf{without replacement} fashion. Hence each element in $\SM_{t+1}$ only occurs once.Then server averages the parameters by $\w_{t+1}^k = \sum_{k \in \SM_{t+1}} p_{k} \frac{N}{K} \v_{t+1}^{k}$. Note that when the $p_k$'s are not all the same, one cannot ensure $\sum_{k \in \SM_{t+1}} p_{k} \frac{N}{K} = 1$.
% \end{enumerate}

% \paragraph{Unbiasedness and bounded variance.}
% Lemma~\ref{lem:conv_v_w_e} shows the mentioned two sampling and averaging schemes are unbiased.
%  In expectation, the next-round parameter (i.e., $\aw_{t+1}$) is equal to the weighted average of parameters in \textbf{all devices} after SGD updates (i.e., $\av_{t+1}$). However, the original scheme in \citep{mcmahan2016communication} (see Table~\ref{tab:conv}) does not enjoy this property. But it is very similar to Scheme II except the averaging scheme. Hence our analysis cannot cover the original scheme.
 
%  Lemma~\ref{lem:conv_v_w} shows the expected difference between $\av_{t+1}$ and $\aw_{t+1}$ is bounded. $\ESt \left\| \av_{t+1} - \aw_{t+1} \right\|^2$ is actually the variance of $\aw_{t+1}$.
 

% \begin{lem}[Unbiased sampling scheme]
% 	\label{lem:conv_v_w_e}
% 	If $t+1 \in \IM_E$, for Scheme I and Scheme II, we have
% 	\[
% 	\ESt (\aw_{t+1}) = \av_{t+1}.
% 	\]
% \end{lem}


% \begin{lem}[Bounding the variance of $\aw_t$]
% 	\label{lem:conv_v_w}
% 	For $t+1 \in \IM$, assume that $\eta_t$ is non-increasing and $\eta_{t} \le 2 \eta_{t+E}$ for all $t\geq 0$. We have the following results.
% 	\begin{enumerate}[(1)]
% 		\item For Scheme I, the expected difference between $\av_{t+1}$ and $\aw_{t+1}$ is bounded by
% 		\[
% 		\ESt \left\| \av_{t+1} - \aw_{t+1} \right\|^2 \leq \frac{4}{K} \eta_t^2 E^2 G^2.
% 		\]
% 		\item For Scheme II, assuming $p_1=p_2=\cdots=p_N=\frac{1}{N}$, the expected difference between $\av_{t+1}$ and $\aw_{t+1}$ is bounded by
% 		\[
% 		\ESt \left\| \av_{t+1} - \aw_{t+1} \right\|^2 \leq  \frac{N-K}{N-1} \frac{4}{K}\eta_t^2 E^2 G^2.
% 		\]
% 	\end{enumerate}
% \end{lem}



% \subsection{Completing the Proof of Theorem~\ref{thm:w_replace} and \ref{thm:wo_replace}}
% \begin{proof}
% Note that
% \begin{align*}
% \left\| \aw_{t+1} - \w^* \right\|^2  
% &=    \left\| \aw_{t+1} - \av_{t+1} + \av_{t+1} - \w^* \right\|^2 \\
% & = \underbrace{\left\| \aw_{t+1} - \av_{t+1} \right\|^2}_{A_1} +
% \underbrace{\left\| \av_{t+1} - \w^* \right\|^2}_{A_2} +
% \underbrace{2\langle \aw_{t+1} - \av_{t+1} , \av_{t+1} - \w^*  \rangle}_{A_3}.
% \end{align*}	
% When expectation is taken over $\SM_{t+1}$, the last term ($A_3$) vanishes due to the unbiasedness of $\aw_{t+1}$. 

% If $t+1 \notin \IM_E$, $A_1$ vanishes since $\aw_{t+1} = \av_{t+1}$. We use Lemma~\ref{lem:conv_v_w} to bound $A_2$. Then it follows that
% \[  \EB \left\| \aw_{t+1} - \w^* \right\|^2   \leq  (1-\eta_t \mu) \EB \left\|\aw_{t}-\w^{\star}\right\|^{2}  + \eta_t^2 B. \]

% If $t+1 \in \IM_E$, we additionally use Lemma~\ref{lem:conv_v_w} to bound $A_1$. Then
% \begin{align}
% \label{eq:conv_final}
% \EB \left\| \aw_{t+1} - \w^* \right\|^2  
% & = \EB \left\| \aw_{t+1} - \av_{t+1} \right\|^2  + \EB \left\| \av_{t+1} - \w^* \right\|^2 \nonumber \\
% & \leq  (1-\eta_t \mu) \EB \left\|\aw_{t}-\w^{\star}\right\|^{2}  + \eta_t^2 (B+ C),
% \end{align}
% where $C$ is the upper bound of $\frac{1}{\eta_t^2} \ESt \left\| \av_{t+1} - \aw_{t+1} \right\|^2$ ($C$ is defined in Theorem~\ref{thm:w_replace} and~\ref{thm:wo_replace}). 

% The only difference between~\eqref{eq:conv_final} and~\eqref{eq:conv_full_final} is the additional $C$.
% Thus we can use the same argument there to prove the theorems here.
% Specifically, for a diminishing stepsize, $\eta_t = \frac{\beta}{t + \gamma}$ for some $\beta > \frac{1}{\mu}$ and $\gamma > 0$ such that $\eta_1 \le \min\{\frac{1}{\mu}, \frac{1}{4L}\}=\frac{1}{4L}$ and $\eta_{t} \le 2 \eta_{t+E}$, we can prove $\EB \left\| \aw_{t+1} - \w^* \right\|^2   \le \frac{v}{\gamma + t}$ where $v = \max\left\{ \frac{\beta^2 (B+C)}{\beta \mu -1}, (\gamma+1)\|\w_1 -\w^*\|^2\right\}$.

% Then by the strong convexity of $F(\cdot)$,
% \[  \EB [F(\aw_t)] - F^* \le \frac{L}{2} \Delta_t  \le \frac{L}{2} \frac{v}{\gamma + t}.\]
% Specifically, if we choose $\beta = \frac{2}{\mu},\gamma = \max\{8 \frac{L}{\mu}, E\}-1$ and denote $\kappa = \frac{L}{\mu}$, then  $\eta_t = \frac{2}{\mu} \frac{1}{\gamma + t}$ and 
% \[  \EB [F(\aw_t)] - F^* \le   \frac{\kappa}{\gamma + t} \left( \frac{2(B+C)}{\mu} +  \frac{ \mu (\gamma+1)}{2} \|\w_1 -\w^*\|^2 \right). \]
% \end{proof}


% \subsection{Deferred proofs of key lemmas}

% \begin{proof}[Proof of Lemma~\ref{lem:conv_v_w_e}]
% We first give a key observation which is useful to prove the followings. Let $\{x_i\}_{i=1}^N$ denote any fixed deterministic sequence. We sample a multiset $\SM_t$ (with size $K$) by the procedure where
% for each sampling time, we sample $x_k$ with probability $q_k$ for each time. Pay attention that two samples are not necessarily independent. We only require each sampling distribution is identically. Let $\SM_t = \{i_1, \cdots, i_K\} \subset [N]$ (some $i_k$'s may have the same value). Then
% \[  \EB_{\SM_t}  \sumk x_k = \EB_{\SM_t}  \sum_{k=1}^K x_{i_k} = K \EB_{\SM_t}  x_{i_1} = K \sum_{k=1}^Nq_k x_k. \]
% For Scheme I, $q_k = p_k$ and for Scheme II, $q_k = \frac{1}{N}$. It is easy to prove this lemma when equipped with this observation.
% \end{proof}

% \begin{proof}[Proof of Lemma~\ref{lem:conv_v_w}]
% 	We separately prove the bounded variance for two schemes. Let $\SM_{t+1} = \{i_1, \cdots, i_K \} $ denote the multiset of chosen indexes.
	
% 	(1) For Scheme I, $\aw_{t+1} = \frac{1}{K} \sum_{l=1}^K \v_{t+1}^{i_l}$. Taking expectation over $\SM_{t+1}$, we have
	
% 	\begin{equation}
% 	\label{eq:v_s1}
% 	\ESt \left\| \aw_{t+1} - \av_{t+1} \right\|^2 
% = \ESt \frac{1}{K^2} \sum_{l=1}^K \left\| \v_{t+1}^{i_l} - \av_{t+1} \right\|^2 
% =  \frac{1}{K} \sum_{k=1}^N p_k \left\| \v_{t+1}^{k} - \av_{t+1} \right\|^2
% 	\end{equation}
% 	where the first equality follows from $\v_{t+1}^{i_l}$ are independent and unbiased.
	
% 	To bound~\eqref{eq:v_s1}, we use the same argument in Lemma~\ref{lem:conv_v_w}. Since $t+1 \in \IM_E$, we know that the time $t_0 = t - E +1 \in \IM_E$ is the communication time, which implies  $\{\w_{t_0}^k\}_{k=1}^N$ is identical. Then 
% 	\begin{align*}
% 	\myave \left\| \v_{t+1}^{k} - \av_{t+1} \right\|^2 
% 	&=  \myave \left\| (\v_{t+1}^{k} - \aw_{t_0}) - ( \av_{t+1} - \aw_{t_0} ) \right\|^2 \\
% 	&\leq \myave \left\|\v_{t+1}^{k} - \aw_{t_0} \right\|^2
% 	\end{align*}
% 	where the last inequality results from $\myave (\v_{t+1}^k - \aw_{t_0}) = \av_{t+1} - \aw_{t_0}$ and $\EB \| \vx-\EB \vx \|^2 \leq \EB \| \vx \|^2$. Similarly, we have
% 	\begin{align*}
% 	\ESt \left\| \aw_{t+1} - \av_{t+1} \right\|^2 
% 	& \leq \frac{1}{K}   \myave \EB \left\|\v_{t+1}^k - \aw_{t_0} \right\|^2 \\
% 	& \leq \frac{1}{K}   \myave \EB \left\|\v_{t+1}^k - \w_{t_0}^k \right\|^2 \\
% 	& \leq \frac{1}{K} \myave   E \sum_{i=t_0}^t \EB \left\| \eta_i \nabla F_k(\w_i^k, \xi_i^k) \right\|^2 \\
% 	& \leq  \frac{1}{K} E^2 \eta_{t_0}^2 G^2 \leq \frac{4}{K} \eta_t^2 E^2 G^2
% 	\end{align*}
% 	where in the last inequality we use the fact that $\eta_t$ is non-increasing and $\eta_{t_0} \leq 2 \eta_t$.
	
% 	(2) For Scheme II, when assuming $p_{1}=p_{2}=\cdots=p_{N}=\frac{1}{N}$, we again have $\aw_{t+1} = \frac{1}{K} \sum_{l=1}^K \v_{t+1}^{i_l}$.
	
% 	\begin{align*}
% 	\ESt& \left\| \aw_{t+1} - \av_{t+1} \right\|^2 = \ESt \left\| \frac{1}{K} \sum_{i \in S_{t+1}} \v_{t+1}^i - \av_{t+1} \right\|^2 = \frac{1}{K^2} \ESt \left\|  \sum_{i=1}^N \IB{i \in S_t} (\v_{t+1}^i - \av_{t+1}) \right\|^2\\
% 	& = \frac{1}{K^2} \left[\sum_{i \in [N]}
% 	\PB\left(i \in S_{t+1}\right) \left\|  \v_{t+1}^i - \av_{t+1} \right\|^2 +
% 	\sum_{i\ne j} \PB\left( i,j \in S_{t+1}\right) \langle  \v_{t+1}^i - \av_{t+1} , \v_{t+1}^j - \av_{t+1} \rangle 
% 	\right]\\
% 	& = \frac{1}{KN}  \sum_{i=1}^N   \left\|  \v_{t+1}^i - \av_{t+1} \right\|^2 
% 	+ \sum_{i\ne j} \frac{K-1}{KN(N-1)}  \langle  \v_{t+1}^i - \av_{t+1} , \v_{t+1}^j - \av_{t+1}\rangle  \\
% 	& = \frac{1}{K(N-1)}\left(1-\frac{K}{N}\right) \sum_{i=1}^N \left\| \v_{t+1}^i - \av_{t+1} \right\|^2
% 	\end{align*}
% 	where we use the following equalities: (1) $\PB\left(i \in S_{t+1}\right) = \frac{K}{N}$ and $ \PB\left( i,j \in S_{t+1}\right) = \frac{K(K-1)}{N(N-1)}$ for all $i \ne j$ and (2)  $\sum_{i \in [N]} \left\|  \v_{t+1}^i - \av_{t+1} \right\|^2 +
% 	\sum_{i\ne j}  \langle  \v_{t+1}^i - \av_{t+1} , \v_{t+1}^j - \av_{t+1}\rangle = 0$.
	
% 	Therefore,
% 	\begin{align*}
% 	\EB \left\| \aw_{t+1} - \av_{t+1} \right\|^2 
% 	& =  \frac{N}{K(N-1)}\left(1-\frac{K}{N}\right) \EB\left[ \frac{1}{N} \sum_{i=1}^N \left\| \v_{t+1}^i - \av_{t+1} \right\|^2 \right] \\
% 	& \leq \frac{N}{K(N-1)}\left(1-\frac{K}{N}\right) \EB\left[ \frac{1}{N} \sum_{i=1}^N \left\| \v_{t+1}^i - \aw_{t_0} \right\|^2 \right] \\
% 	& \leq \frac{N}{K(N-1)}\left(1-\frac{K}{N}\right) 4 \eta_t^2 E^2 G^2.
% 	\end{align*}
% 	where in the last inequality we use the same argument in (1).
% \end{proof}

% \begin{table*}[]

% \caption{Test accuracy of average and large models. Left side of the item represents the average accuracy of models at 25\%, 50\%, and 100\%; right side of the item represents the accuracy of 100\% models. Best results are shown in blod.}
% \label{Table: Experiment}
% \scriptsize
% \begin{tabular}{cc|ccc|ccc|ccc|c|ccc}
% \hline
% \multirow{2}{*}{Model}       & \multirow{2}{*}{Algorithm} & \multicolumn{3}{c|}{CIFAR10}                                       & \multicolumn{3}{c|}{CIFAR100}                                      & \multicolumn{3}{c|}{TinyImagenet}                                  & FEMNIST              & \multicolumn{3}{c}{WIDAR}                                          \\ \cline{3-15} 
%                              &                            & IID                  & $\alpha = 0.6$       & $\alpha = 0.3$       & IID                  & $\alpha = 0.6$       & $\alpha = 0.3$       & IID                  & $\alpha = 0.6$       & $\alpha = 0.3$       & -                    & IID                  & $\alpha = 0.6$       & $\alpha = 0.3$       \\ \hline
% \multirow{4}{*}{VGG16}       & Decoupled                  & 75.81 72.76          & 73.57 69.91          & 69.95 66.01          & 34.53 29.44          & 33.68 29.12          & 33.33 28.77          & 25.62 21.14          & 26.56 22.53          & 26.70 23.51          & 78.70 71.63          & 67.51 60.80          & 66.41 60.28          & 64.12 58.47          \\
%                              & HeteroFL                   & 79.75 76.92          & 77.53 75.45          & 73.89 71.50          & 34.37 29.92          & 35.02 31.31          & 35.43 31.56          & 25.51 23.19          &                      &                      & \textbf{79.84 72.54} & 70.81 67.35          & 68.82 64.90          & \textbf{67.28 64.11} \\
%                              & ScaleFL                    & 80.36 77.72          & 75.99 74.00          & 72.95 69.87          & 34.10 29.00          & 34.26 29.38          & 33.60 29.18          & 22.37 19.38          & 23.15 20.96          & 24.67 21.62          & 70.85 63.61          & 69.99 67.80          & 68.42 65.95          & 64.50 62.99          \\
%                              & FlexFL                         & \textbf{84.75 85.16} & \textbf{83.11 83.45} & \textbf{80.60 81.06} & \textbf{40.27 40.35} & \textbf{41.29 41.30} & \textbf{39.55 39.99} & \textbf{26.61 26.97} & \textbf{29.19 29.56} & \textbf{31.07 31.42} & 77.16 75.94          & \textbf{71.66 72.13} & \textbf{71.04 70.92} & 67.20 68.11          \\ \hline
% \multirow{4}{*}{Resnet34}    & Decoupled                  & 62.92 56.97          & 59.01 54.11          & 55.35 51.32          & 26.88 22.28          & 26.68 22.01          & 25.24 19.81          & 33.13 29.07          &                      &                      & 74.02 64.27          & 63.54 58.36          & 60.65 54.89          & 58.84 53.84          \\
%                              & HeteroFL                   & 69.56 63.17          & 65.14 61.25          & 61.29 57.02          & 31.79 24.52          & 31.01 25.37          & 30.92 24.68          & 38.35 31.90          &                      &                      & 76.99 68.07          & 67.90 63.05          & 65.17 60.59          & 59.83 56.71          \\
%                              & ScaleFL                    & 76.65 74.23          & 71.57 68.50          & 66.56 61.67          & 36.84 31.87          & 34.95 29.51          & 32.81 27.50          & 38.31 32.84          & 36.68 31.32          & 36.02 31.77          & 76.94 69.25          & 64.77 61.17          & 61.44 58.92          & 58.97 57.67          \\
%                              & FlexFL                         & \textbf{77.48 78.06} & \textbf{72.89 73.71} & \textbf{69.08 69.60} & \textbf{37.76 37.38} & \textbf{37.63 37.31} & \textbf{37.34 37.38} & \textbf{40.53 40.85} & 38.64 38.32          & 37.89 37.88          & \textbf{83.64 80.46} & \textbf{72.43 73.10} & \textbf{71.19 71.57} & \textbf{67.91 68.77} \\ \hline
% \multirow{4}{*}{MobileNetV2} & Decoupled                  & 53.01 52.03          & 48.34 47.71          & 42.42 40.29          & 20.20 17.74          & 20.74 18.08          & 20.22 17.58          & 21.57 16.11          & 20.34 17.60          & 20.11 16.35          & 68.40 56.33          & 51.28 44.45          & 45.92 44.04          & 43.76 38.92          \\
%                              & HeteroFL                   & 57.60 52.69          & 51.31 48.33          & 44.00 40.16          & 23.49 19.31          & 22.60 19.20          & 21.60 17.80          & 24.96 20.05          &                      &                      & 70.94 61.87          & 56.49 53.05          & 51.74 49.15          & 47.67 45.02          \\
%                              & ScaleFL                    & 63.42 59.83          & 54.57 48.77          & 49.90 45.10          & 26.53 21.72          & 25.09 19.90          & 24.30 18.24          & 26.64 23.63          & 26.31 23.43          & 24.69 22.25          & 71.38 62.02          & 58.17 55.01          & 53.13 47.45          & 46.93 44.12          \\
%                              & FlexFL                         & \textbf{68.47 69.18} & \textbf{60.00 61.32} & \textbf{56.87 58.23} & \textbf{29.11 28.30} & \textbf{27.86 27.14} & \textbf{26.78 26.41} & \textbf{28.26 27.44} & \textbf{27.46 25.55} & \textbf{25.38 24.00} & \textbf{77.25 71.38} & \textbf{64.92 65.67} & \textbf{63.43 63.98} & \textbf{57.61 59.26} \\ \hline
% \end{tabular}
% \end{table*}
